# Supplementary material for: Non-Hermitian bulk-boundary correspondence and auxiliary generalized Brillouin zone theory
Source: arXiv:1912.05499 source file (2020-10-30)
Supplement: Supplementary file 1 [file SM_v1.pdf]

# Supplemental Material for “Auxiliary generalized Brillouin zone method in non-Hermitian band theory”

Zhesen Yang,<sup>1,2,\*</sup> Kai Zhang,<sup>1,2,\*</sup> Chen Fang,<sup>1,†</sup> and Jiangping Hu<sup>1,3,4,‡</sup>

<sup>1</sup>*Beijing National Laboratory for Condensed Matter Physics,  
and Institute of Physics, Chinese Academy of Sciences, Beijing 100190, China*

<sup>2</sup>*University of Chinese Academy of Sciences, Beijing 100049, China*

<sup>3</sup>*Kavli Institute for Theoretical Sciences and CAS Center for Excellence in Topological Quantum Computation,  
University of Chinese Academy of Sciences, Beijing 100190, China*

<sup>4</sup>*South Bay Interdisciplinary Science Center, Dongguan, Guangdong Province, China*

## Contents

|                                                       |   |
|-------------------------------------------------------|---|
| <b>I. An exact solvable model</b>                     | 1 |
| A. Open boundary( $\lambda = 0$ ) solution            | 2 |
| B. Periodic boundary ( $\lambda = 1$ ) solution       | 3 |
| <b>II. GBZ condition</b>                              | 4 |
| <b>III. Characteristic equation of Hermitian case</b> | 5 |
| <b>IV. Resultant of two polynomials</b>               | 5 |
| <b>V. Numerical result of Fig. 1</b>                  | 7 |
| <b>VI. Single band model</b>                          | 7 |
| <b>References</b>                                     | 7 |

## I. AN EXACT SOLVABLE MODEL

In this section, we will use an exact solvable model to illustrate the procedure of exact solution for a finite size lattice system with open boundary condition. Consider the following Hamiltonian with arbitrary boundary condition

$$\begin{aligned}\hat{H}(\lambda) &= \hat{H}_0 + \lambda \hat{H}_B, \\ \hat{H}_0 &= \sum_{i=1}^{N-1} (t_1 \hat{c}_i^\dagger \hat{c}_{i+1} + t_{-1} \hat{c}_{i+1}^\dagger \hat{c}_i), \\ \hat{H}_B &= t_{-1} \hat{c}_1^\dagger \hat{c}_N + t_1 \hat{c}_N^\dagger \hat{c}_1,\end{aligned}\tag{1}$$

where  $\hat{H}_0$  is the open boundary Hamiltonian and  $N$  denotes the number of sites of the one dimensional chain. In order to simplify the discussion, we can assume that  $t_{\pm 1}$  are real positive numbers without loss of generality. If  $t_1 = t_{-1}^*$  and  $\lambda \in \mathbb{R}$ ,  $\hat{H}(\lambda)$  is Hermitian, otherwise, it is non-Hermitian. The eigenequation of the Hamiltonian in Eq. (1) can

---

\*These two authors contributed equally

†Electronic address: [cfang@iphy.ac.cn](mailto:cfang@iphy.ac.cn)

‡Electronic address: [jphu@iphy.ac.cn](mailto:jphu@iphy.ac.cn)

be written as the following matrix form,

$$\begin{pmatrix} 0 & t_1 & 0 & \dots & 0 & \lambda t_{-1} \\ t_{-1} & 0 & t_1 & \dots & 0 & 0 \\ 0 & t_{-1} & 0 & \dots & 0 & 0 \\ \vdots & \vdots & \vdots & \ddots & \vdots & \vdots \\ 0 & 0 & 0 & \dots & 0 & t_1 \\ \lambda t_1 & 0 & 0 & \dots & t_{-1} & 0 \end{pmatrix} \begin{pmatrix} \phi_1 \\ \phi_2 \\ \phi_3 \\ \vdots \\ \phi_{N-1} \\ \phi_N \end{pmatrix} = E \begin{pmatrix} \phi_1 \\ \phi_2 \\ \phi_3 \\ \vdots \\ \phi_{N-1} \\ \phi_N \end{pmatrix}, \quad (2)$$

where  $\Phi = (\phi_1, \dots, \phi_N)^t$  represents the non-normalized eigenfunction of  $\hat{H}(\lambda)$ .

### A. Open boundary( $\lambda = 0$ ) solution

If  $\lambda = 0$ , the Hamiltonian reduces to the case of open boundary. The procedure to obtain the solution is similar to the case of solving the infinite square well problem, where we first solve the (bulk) Schrödinger equation  $-\hbar^2 \partial_x^2 \phi(x) = 2m(E - V_0)\phi(x)$  and eigenstates can be expressed as the superposition of (bulk) solutions  $\phi(x) = e^{\pm i k x}$  such as the boundary condition is satisfied.

Based on the same method, the recursive bulk equation can be obtained from Eq. (2),

$$t_{-1}\phi_{i-1} + t_1\phi_{i+1} = E\phi_i, \quad (3)$$

where  $i = 2, \dots, N-1$ . We first solve the bulk equation. Notice that Eq. (3) has discrete translational symmetry. This implies the bulk solution can be written as  $\Phi(\beta) = (\beta^1, \beta^2, \dots, \beta^N)^t$ . Putting this solution into Eq. (3), the bulk equation becomes

$$t_1\beta^2 - E\beta + t_{-1} = 0. \quad (4)$$

Hence, for a given  $E$ , there exist two bulk solutions,  $\Phi_E(\beta_1)$  and  $\Phi_E(\beta_2)$ , where

$$\beta_{1/2} = \frac{E \pm \sqrt{E^2 - 4t_1 t_{-1}}}{2t_1}. \quad (5)$$

Next, the discussion can be classified by the following two cases.

(a).  $\beta_1 \neq \beta_2$  case

If  $\beta_1 \neq \beta_2$ , the solution of Eq. 2 with eigenvalue  $E$  can be written as the superposition of the above two bulk solutions, namely,

$$\Phi_E = c_1 \Phi_E(\beta_1) + c_2 \Phi_E(\beta_2). \quad (6)$$

Putting Eq. (6) into Eq. (2), one can obtain the following constraint of boundary condition

$$\begin{aligned} t_1(c_1\beta_1^2 + c_2\beta_2^2) &= E(c_1\beta_1 + c_2\beta_2), \\ t_{-1}(c_1\beta_1^{N-1} + c_2\beta_2^{N-1}) &= E(c_1\beta_1^N + c_2\beta_2^N). \end{aligned} \quad (7)$$

By solving this boundary condition, one can obtain a set of quantized  $\beta$  and  $E$  for a finite size system. Using the bulk equation Eq. (4), the above boundary condition Eq. (7) can be rewritten as the following matrix form,

$$\begin{pmatrix} t_1\beta_1^2 - (t_{-1} + t_1\beta_1^2) & t_1\beta_2^2 - (t_{-1} + t_1\beta_2^2) \\ t_{-1}\beta_1^{N-1} - (t_{-1}\beta_1^{N-1} + t_1\beta_1^{N+1}) & t_{-1}\beta_2^{N-1} - (t_{-1}\beta_2^{N-1} + t_1\beta_2^{N+1}) \end{pmatrix} \begin{pmatrix} c_1 \\ c_2 \end{pmatrix} = \begin{pmatrix} -t_{-1} & -t_{-1} \\ -t_1\beta_1^{N+1} & -t_1\beta_2^{N+1} \end{pmatrix} \begin{pmatrix} c_1 \\ c_2 \end{pmatrix} = 0. \quad (8)$$

The nontrivial solutions require the determinant of the coefficient matrix vanish, namely,

$$t_1 t_{-1} (\beta_2^{N+1} - \beta_1^{N+1}) = 0. \quad (9)$$

Using the condition  $\beta_1\beta_2 = t_{-1}/t_1$  from Eq. (4), one can obtain

$$(t_{-1}/t_1)^{N+1} - \beta_{1/2}^{2N+2} = 0, \quad (10)$$

where  $\beta_{1/2}$  represents  $\beta_1$  and  $\beta_2$ . By solving the above equation, one can obtain the following quantized  $\beta_{1/2}$

$$\beta_{1/2} = \left(\frac{t_{-1}}{t_1}\right)^{1/2} e^{ik}, \quad \beta_{2/1} = \left(\frac{t_{-1}}{t_1}\right)^{1/2} e^{-ik}, \quad (11)$$

and  $E$ ,

$$E = t_0 + 2\sqrt{t_1 t_{-1}} \cos k, \quad (12)$$

where

$$k = \frac{\pi m}{N+1}, \quad m = 1, \dots, N \quad (13)$$

Notice that  $m \neq 0, \pm(N+1)$ , since we forbid the case  $\beta_1 = \beta_2$ .

(b).  $\beta_1 = \beta_2$  case

If  $\beta_1 = \beta_2$ , the solution can not be written as the form of Eq. (6). According to Eq. (5),  $\beta_1 = \beta_2$  requires

$$E_c = t_0 \pm 2\sqrt{t_1 t_{-1}}, \quad (14)$$

and

$$\beta_c = \beta_1 = \beta_2 = \pm\sqrt{t_{-1}/t_1} = \sqrt{t_{-1}/t_1} e^{ik_c}, \quad (15)$$

where  $k_c = 0, \pm\pi$ . If  $N$  is finite, this bulk wave function  $\Phi_{E_c}(\beta_c)$  do not satisfy the boundary condition Eq. (7). However, if  $N \rightarrow \infty$ , there exist two different cases: (i)  $|\beta| = 1$ , namely the Hermitian case ( $t_{-1} = t_1$  since we have already assumed  $t_{\pm 1}$  are real positive numbers), the bulk solution  $\Phi_{E_c}(\beta_c) = e^{ik_c x}$  is the Bloch wave function, which becomes the asymptotic solution in the  $N \rightarrow \infty$  limit; (ii)  $|\beta| \neq 1$ , which is the non-Hermitian case ( $t_{-1} \neq t_1$ ), the bulk solution  $\Phi_{E_c}(\beta_c) = \sqrt{t_{-1}/t_1} e^{ik_c x}$  will be divergent at the infinity boundary. Hence, they can not be the (bounded) asymptotic solutions.

By solving the coefficients  $c_1$  and  $c_2$  from Eq. (8), The eigenfunctions can be obtained

$$\Phi_E \propto \Phi_E(\beta_1) - \Phi_E(\beta_2) \propto (\phi_1, \dots, \phi_N)^t, \quad (16)$$

with

$$\phi_m = \left(\frac{t_{-1}}{t_1}\right)^{m/2} \sin km, \quad (17)$$

where  $k = m\pi/(N+1)$  and  $m = 1, \dots, N$ . If  $t_1 \neq t_{-1}$ , all the eigenstates of the Hamiltonian will be localized at one of the boundary of the lattice chain. These eigenstates are dubbed as non-Hermitian skin modes [1].

## B. Periodic boundary ( $\lambda = 1$ ) solution

As a comparison, we use the same method to solve Eq. (2) with periodic boundary condition, namely,  $\lambda = 1$ . It can be shown, the boundary condition in this case becomes

$$\mathcal{M}_B \begin{pmatrix} c_1 \\ c_2 \end{pmatrix} = \begin{pmatrix} 1 - \beta_1^N & 1 - \beta_2^N \\ \beta_1(1 - \beta_1^N) & \beta_2(1 - \beta_2^N) \end{pmatrix} \begin{pmatrix} c_1 \\ c_2 \end{pmatrix} = 0. \quad (18)$$

One can notice the boundary condition is independent of the parameter. The condition for the vanishing of the determinant of the coefficient matrix can be written as

$$(\beta_1 - \beta_2)(1 - \beta_1^N)(1 - \beta_2^N) = 0. \quad (19)$$

This equation requires

$$\beta_{1/2} = e^{ik}, \quad k = \frac{2\pi m}{N}, \quad (20)$$

A little difference occurs between the Hermitian and non-Hermitian case.

(a).  $t_1 = t_{-1}$  case

In this Hermitian case, according to  $\beta_1\beta_2 = t_{-1}/t_1 = 1$ , both  $\Psi_E(\beta_1)$  and  $\Psi_E(\beta_2)$  are the solutions. And any linear superposition of them is also the solution.

(b).  $t_1 \neq t_{-1}$  case

In this non-Hermitian case, according to  $\beta_1\beta_2 = t_{-1}/t_1 \neq 1$ , either  $\Psi_E(\beta_1)$  or  $\Psi_E(\beta_2)$  is the solutions. Their linear superposition  $c_1\Psi_E(\beta_1) + c_2\Psi_E(\beta_2)$  is not the solution. This means for a give energy, there only exist one eigenstates in the case of periodic boundary condition. It has been shown that this implies the nontrivial winding of energy and the failure of conventional bulk-boundary correspondence [2, 3].

## II. GBZ CONDITION

The condition of GBZ has been first explored in Ref [1, 4] with chiral symmetry and in Ref [2] with general single band models. Here we generalize the condition of GBZ to arbitrary multi-band models without any symmetry or with chiral symmetry.

Consider a general  $m$ -band 1D Hamiltonian in real space

$$\hat{H} = \sum_{i,j=1}^N \sum_{\mu,\nu=1}^m t_{ij}^{\mu\nu} \hat{c}_{i\mu}^\dagger \hat{c}_{j\nu}, \quad (21)$$

where  $t_{ij}^{\mu\nu} \neq (t_{ji}^{\nu\mu})^*$  and  $i, j$  and  $\mu, \nu$  label the lattice sites and band indexes respectively.

Firstly, the characteristic equation can be written as

$$f(\beta, E) = \det[\mathcal{H}(\beta) - E\hat{I}] = \sum_{i=-p}^s \sum_{j=0}^m c_{ij} \beta^i E^j = 0, \quad (22)$$

where  $[\mathcal{H}(\beta)]_{\mu\nu} = \sum_{l=-l_1}^{l_2} t_l^{\mu\nu} \beta^l$ ,  $t_l^{\mu\nu} = t_{ij}^{\mu\nu} \delta_{i+l,j}$ , and  $\beta = e^{ik}$  labeling the Bloch wave with the complex wave-vector  $k$ . Secondly,

- if  $f(\beta, E)$  is an irreducible algebraic polynomial, we can solve the characteristic equation for a given  $E$ , and order the solutions by the absolute value as

$$|\beta_1(E)| \leq |\beta_2(E)| \leq \dots \leq |\beta_{p+s}(E)|. \quad (23)$$

Finally, if  $|\beta_p(E)| = |\beta_{p+1}(E)|$ , where  $p$  is the order of the pole in Eq. (22), then,  $E$  is an eigenvalue of  $\hat{H}$  in the thermodynamic limit  $N \rightarrow \infty$ .

- if  $f(\beta, E)$  is an reducible algebraic polynomial, which can be written as

$$f(\beta, E) = \prod_{i=1}^n f_i(\beta, E), \quad (24)$$

where  $f_i(\beta, E)$  is irreducible algebraic polynomial, then, for every  $i = 1, \dots, n$  we can solve  $f_i(\beta, E) = 0$  for a given  $E$ , and order the corresponding solutions by the absolute value as

$$|\beta_{i,1}(E)| \leq |\beta_{i,2}(E)| \leq \dots \leq |\beta_{i,p_i+s_i}(E)|. \quad (25)$$

Finally, if  $|\beta_{i,p_i}(E)| = |\beta_{i,p_i+1}(E)|$ , where  $p_i$  is the order of the pole in  $f_i(\beta, E)$ , then,  $E$  is an eigenvalue of  $\hat{H}$  in the thermodynamic limit  $N \rightarrow \infty$ .

The second case of the above discussion applies to the cases where several bands are independent and not be coupled together. The proof for the first case can be found in the Ref [2, 4]. Here we complete the condition in second case, which can be viewed as a generalization of the first case. The example can be found in the main text.

### III. CHARACTERISTIC EQUATION OF HERMITIAN CASE

For the Hamiltonian with open boundary condition defined in Eq. 1 in the main text, if the Hamiltonian is Hermitian, it must satisfy

$$H^* = H^t. \quad (26)$$

Here we define

$$H_1 := H^*, \quad H_2 := H^t \quad (27)$$

Then, the corresponding bulk Hamiltonians can be written as

$$[\mathcal{H}_1(\beta)]_{\mu\nu} = \sum_{\langle i,j \rangle} (t_{ij}^{\mu\nu})^* \beta^{j-i} = \sum_{l=-l_1}^{l_2} (t_l^{\mu\nu})^* \beta^l, \quad (28)$$

and

$$[\mathcal{H}_2(\beta)]_{\mu\nu} = \sum_{\langle i,j \rangle} t_{ji}^{\mu\nu} \beta^{j-i} = \sum_{l=-l_1}^{l_2} t_l^{\mu\nu} \beta^{-l}. \quad (29)$$

Now, the characteristic equation for the  $H_1$  and  $H_2$  becomes

$$\det[\mathcal{H}_1(\beta) - E\hat{I}] = \sum_{i=-p}^s \sum_{j=0}^m c_{ij}^* \beta^i E^j = f^*(\beta^*, E) = 0, \quad (30)$$

and

$$\det[\mathcal{H}_2(\beta) - E\hat{I}] = \sum_{i=-p}^s \sum_{j=0}^m c_{ij} \beta^{-i} E^j = f(\beta^{-1}, E) = 0, \quad (31)$$

Here we have used the fact that  $E \in \mathbb{R}$  for the Hermitian case. As a result, we obtain

$$f^*(\beta^*, E) = f(1/\beta, E) \quad (32)$$

for the Hermitian Hamiltonian. Notice we want to use the above equation to show that  $C_\beta = e^{ik}$  in the Hermitian case. It is necessary to assume  $\beta^* \neq \beta^{-1}$  in the above derivation.

### IV. RESULTANT OF TWO POLYNOMIALS

In the main text, we have mentioned that the aGBZ can be calculated from the resultant of two polynomials. Now we show how can we calculate them.

**Definition A.1** (Polynomial). A polynomial  $f(x) \in F[x]$  is defined as

$$f(x) = \prod_{i=1}^n (x - \xi_i) = a_n x^n + a_{n-1} x^{n-1} + \dots + a_1 x + a_0, \quad a_n \neq 0 \quad (33)$$

where each coefficient  $a_i$  belongs to the field  $F$  and each root  $\xi_i$  belongs to the extension of  $F$ . For example, if  $a_n, \dots, a_0$  are real numbers,  $\xi_1, \dots, \xi_n$  are complex numbers.

**Definition A.2** (Resultant). Given two polynomials  $f(x) = a_n x^n + \dots + a_0$ ,  $g(x) = b_m x^m + \dots + b_0 \in F[x]$ , their resultant relative to the variable  $x$  is a polynomial over the field of coefficients of  $f(x)$  and  $g(x)$ , and is defined as

$$R(f, g) = a_n^m b_m^n \prod_{i,j} (\xi_i - \eta_j), \quad (34)$$

where  $f(\xi_i) = 0$  for  $1 \leq i \leq n$  and  $g(\eta_j) = 0$  for  $1 \leq j \leq m$ .

**Theorem A.3.** Let  $f(x) = a_n x^n + \dots + a_0$ ,  $g(x) = b_m x^m + \dots + b_0 \in F[x]$ ,

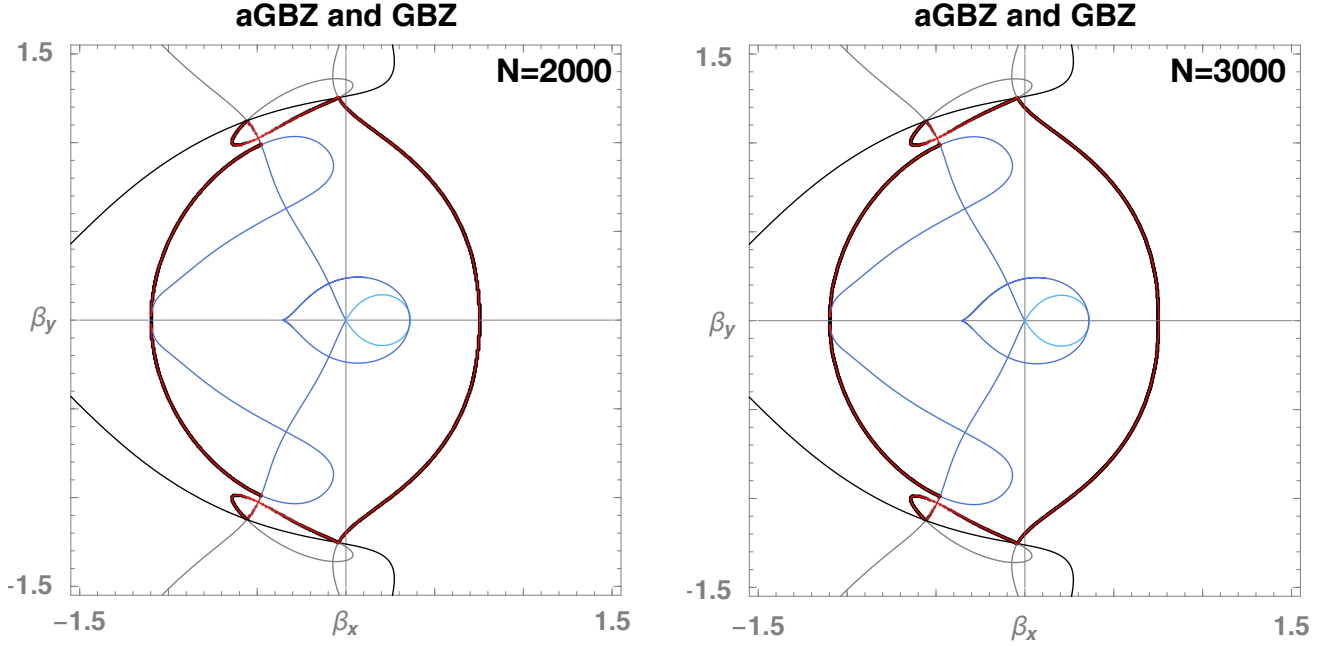

FIG. 1: The numerical results of Fig. 1 in the main text. Here the lattice size ( $N$ ) and degrees of precision ( $P$ ) is chosen to be  $N = 2000$   $P = 800$  for the left and  $N = 3000$   $P = 1800$  for the right. The calculation time for the right side is 11 days. Notice we still do not know whether there exist self-intersection points through the numerical calculation. Here  $\beta_x := \text{Re } \beta$  and  $\beta_y := \text{Im } \beta$ .

1. Suppose that  $f$  has  $n$  roots  $\xi_1, \dots, \xi_n$  in some extension of  $F$ . Then

$$R(f, g) = a_n^m \prod_{i=1}^n g(\xi_i). \quad (35)$$

2. Suppose that  $g$  has  $m$  roots  $\eta_1, \dots, \eta_m$  in some extension of  $F$ . Then

$$R(f, g) = (-1)^{mn} b_m^n \prod_{j=1}^m f(\eta_j). \quad (36)$$

The proof can be found in Ref [5, 6].

**Theorem A.4.** Let  $f$  and  $g$  be two non-zero polynomials with coefficients in a field  $F$ . Then  $f$  and  $g$  have a common root in some extension of  $F$  if and only if their resultant  $R(f, g)$  is equal to zero.

*Proof:* Suppose  $\gamma$  is their common root,  $R(f, g) \propto (\gamma - \gamma) = 0$ . Conversely, If  $R(f, g) = 0$ , at least one of the factors of  $R(f, g)$  must be zero, say  $\xi_i - \eta_j = 0$ , then,  $\xi_i = \eta_j$  is their common root.

From Theorem A.4, the resultant can be applied to make sure whether or not two polynomials share a common root. However, from Definition A.2, the calculation of the resultant requires to know the roots of each polynomial. The following theorem enables us to calculate the resultant directly according to the coefficients of  $f$  and  $g$ .

**Definition A.5.** The Sylvester matrix of two polynomials  $f(x) = a_n x^n + \dots + a_0$ ,  $g(x) = b_m x^m + \dots + b_0 \in F[x]$  is

defined by

$$\text{Syl}(f, g) = \begin{pmatrix} a_n & a_{n-1} & a_{n-2} & \cdots & 0 & 0 & 0 \\ 0 & a_n & a_{n-1} & \cdots & 0 & 0 & 0 \\ \vdots & \vdots & \vdots & & \vdots & \vdots & \vdots \\ 0 & 0 & 0 & \cdots & a_1 & a_0 & 0 \\ 0 & 0 & 0 & \cdots & a_2 & a_1 & a_0 \\ b_m & b_{m-1} & b_{m-2} & \cdots & 0 & 0 & 0 \\ 0 & b_m & b_{m-1} & \cdots & 0 & 0 & 0 \\ \vdots & \vdots & \vdots & & \vdots & \vdots & \vdots \\ 0 & 0 & 0 & \cdots & b_1 & b_0 & 0 \\ 0 & 0 & 0 & \cdots & b_2 & b_1 & b_0 \end{pmatrix}, \quad (37)$$

where  $a_n, \dots, a_0$  are the coefficients of  $f$  and  $b_m, \dots, b_0$  are the coefficients of  $g$ .

**Theorem A.6.** *The resultant of two polynomials  $f, g$  equals to the determinant of their Sylvester matrix, namely*

$$R(f, g) = \det[\text{Syl}(f, g)] \quad (38)$$

For example, if  $n = 3, m = 2$ ,

$$R(f, g) = \det \begin{pmatrix} a_3 & a_2 & a_1 & a_0 & 0 \\ 0 & a_3 & a_2 & a_1 & a_0 \\ b_2 & b_1 & b_0 & 0 & 0 \\ 0 & b_2 & b_1 & b_0 & 0 \\ 0 & 0 & b_2 & b_1 & b_0 \end{pmatrix}. \quad (39)$$

The proof of this theorem can be found in Ref [5, 6].

## V. NUMERICAL RESULT OF FIG. 1

In this section, we show some additional numerical results of Fig. 1 in the main text. On the left side of Fig. 1, we numerically solve the open boundary Hamiltonian with  $N = 2000$  and 800 degrees of precision in Mathematica. The calculation time is about 3 days. On the right side of Fig. 1, we numerically solve the open boundary Hamiltonian with  $N = 3000$  and 1800 degrees of precision in Mathematica. The calculation time is about 11 days. Even in the right side of Fig. 1, we still do not know whether there exist self-intersection points on the GBZ.

## VI. SINGLE BAND MODEL

Here we will provide some additional examples for the single band model, where the characteristic equation is

$$f(\beta, E) = E - \sum_{m=-p}^s t_m \beta^m, \quad j = 1, 2. \quad (40)$$

To simplify the discussion, we assume that all the parameters are real. Fig. 2 shows some examples of aGBZ and GBZ. The nonzero parameters are chosen to be  $t_{-2} = 1/5, t_{-1} = 3/2, t_1 = 1$  for (a);  $t_{-2} = 1/5, t_{-1} = 1, t_1 = 1, t_2 = 1/3$  for (b);  $t_{-3} = -1/2, t_{-2} = 1/5, t_{-1} = 3/2, t_1 = 1, t_2 = 1/6$  for (c);  $t_{-3} = -1/2, t_{-2} = 1/5, t_{-1} = 3/2, t_1 = 1, t_2 = 1/6, t_3 = 1/2$  for (d). As a comparison, we also plot the numerical calculation of the GBZ in (a1)-(d1) with the gray points, whose size is proportional to  $|\text{Im } E|$ . Any arcs containing the degenerate points satisfying  $\beta_p = \beta_{p+1}$  (red points) must form the GBZ. The eigenvalues are shown in (a2)-(d2)

- 
- [1] S. Yao and Z. Wang, *Phys. Rev. Lett.* **121**, 086803 (2018).
  - [2] K. Zhang, Z. Yang, and C. Fang, [arXiv:1910.01131](#).
  - [3] N. Okuma, K. Kawabata, K. Shiozaki, and M. Sato, [arXiv:1910.02878](#).
  - [4] K. Yokomizo and S. Murakami, *Phys. Rev. Lett.* **123**, 066404 (2019).
  - [5] H. Woody, *Polynomial Resultants*, 10 (2016).
  - [6] S. Janson, *RESULTANT AND DISCRIMINANT OF POLYNOMIALS*, 18 (2010).

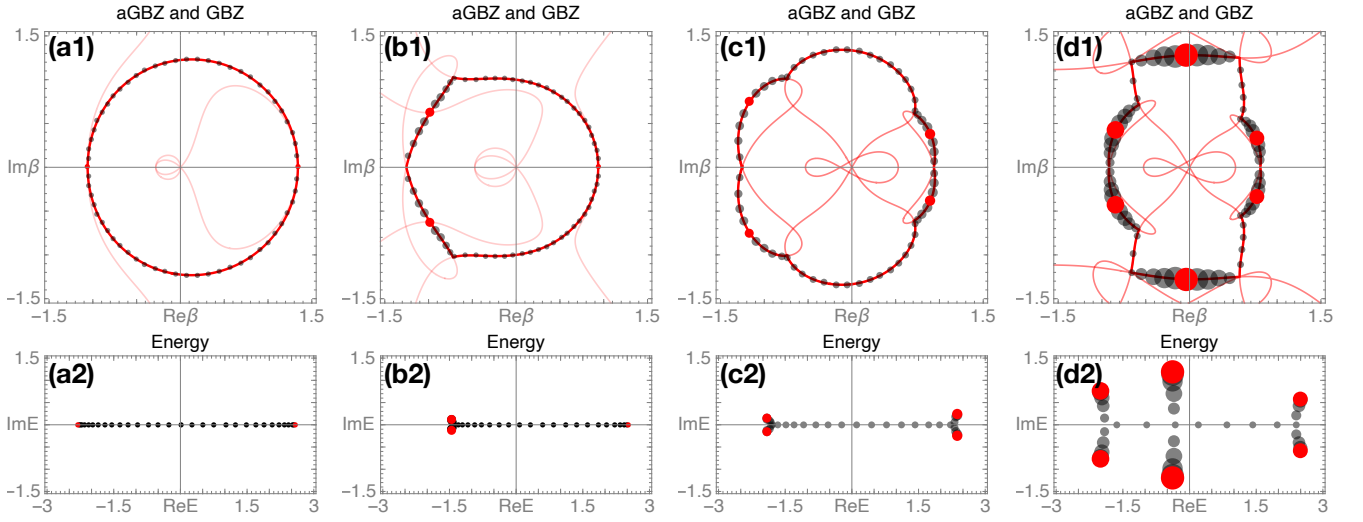

FIG. 2: The GBZ, aGBZ and the corresponding open boundary energy spectra of the Hamiltonian determined by the characteristic equation Eq. 40. In (a1)-(d1), the red curves, gray points, and red points represent the aGBZ, numerical calculation of GBZ with ( $N = 30$ ), and degenerate points satisfying  $\beta_p = \beta_{p+1}$ . The size of the dots is proportional to  $|\text{Im} E|$ . The analytic arcs containing the red points in the aGBZ must form the GBZ. The energy spectrum with  $N = 30$  are plotted in the second row. The model is shown in Eq. (40) and the parameters are chosen to be  $t_{-2} = 1/5, t_{-1} = 3/2, t_1 = 1$  for (a);  $t_{-2} = 1/5, t_{-1} = 1, t_1 = 1, t_2 = 1/3$  for (b);  $t_{-3} = -1/2, t_{-2} = 1/5, t_{-1} = 3/2, t_1 = 1, t_2 = 1/6$  for (c);  $t_{-3} = -1/2, t_{-2} = 1/5, t_{-1} = 3/2, t_1 = 1, t_2 = 1/6, t_3 = 1/2$  for (d).
